# Supplementary material for: An information-theoretic lower bound in time-uniform estimation
Source: arXiv:2402.08794 source file (2024-06-11)
Supplement: Supplementary file 1 [file additional-proofs.tex]

\section{Proof of Lemma~\ref{lemma:kl-cond-bd}}\label{sec:kl-cond-bd}
\begin{proof}
  Let $p, q$ be the densities of $P$ and $Q$ respectively with respect to a
  dominating measure $\mu$.
  Then it is clear that $dP_S/d\mu = \frac{1}{P(S)}p1_S$ and $dQ_S/d\mu = \frac{1}{Q(S)}q1_S$.
  Thus,
  \begin{align*}
    \dkl{P_S}{Q_S}
    &= \int \frac{p}{P(S)}1_S \log\left(\frac{p/P(S)}{q/Q(S)}\right) d\mu \\
    &= \frac{1}{P(S)} \int p\log(p/q)1_S d\mu + \log(Q(S)/P(S)) \\
    &= \frac{1}{P(S)}\dkl{P}{Q} + \log(Q(S)/P(S)) + \frac{1}{P(S)}\int p\log(q/p)1_{S^c}d\mu.
  \end{align*}

  Now, $\log(q/p) = \log(1 + (q-p)/p) \leq (q-p)/p$, and so
  \begin{align*}
    \dkl{P_S}{Q_S}
    &\leq \frac{1}{P(S)}\dkl{P}{Q} + \log(Q(S)/P(S)) + \frac{1}{P(S)}\int (q-p)1_{S^c}d\mu \\
    &= \frac{1}{P(S)}\dkl{P}{Q} + \log(Q(S)/P(S)) + \frac{P(S)-Q(S)}{P(S)}.
  \end{align*}
  Using the same inequality as before, $\log(Q(S)/P(S)) \leq (Q(S)-P(S))/P(S)$,
  and so the latter two terms in the above display are collectively at most 0.
  This proves the claim.
\end{proof}

% \begin{lemma}
%   Let $P_1, \dots, P_M$ be distributions over a set $\cX$ such that
%   $\dkl{P_i}{P_j} \leq D$ for all $i,j \in [M]$.
%   Now let $\correctevent_1, \dots, \correctevent_M$ be measurable sets that partition $\cX$.
%   Then $\max_i P_i(\correctevent_i^c) \geq \frac{M-1}{4}\cdot\exp(-2D)$.
% \end{lemma}
% \begin{proof}
%   Define $\alpha = \max_i P_i(\correctevent_i^c)$.
%   If $\alpha \geq \frac{1}{2}$, then there is nothing to show,
%   so assume otherwise.
%   For any $i \neq j$, we then have by (cite second-order hypercontractive paper Lemma 2.1) that
%   \begin{align*}
%     -\log\left(P_j(\correctevent_i)\right)
%     \leq \frac{\dkl{P_i}{P_j}+\log 2}{1-\alpha}
%     \leq 2(D+\log 2).
%   \end{align*}
%   This implies that $P_j(\correctevent_i) \geq \exp(-2(D+\log 2))$ for all $j \neq i$.
%   Summing over $i$, we thus have
%   \begin{align*}
%     P_j(\correctevent_j^c) = \sum_{i\neq j} P_j(\correctevent_i) \geq (M-1)\exp(-2(D+\log 2)).
%   \end{align*}
% \end{proof}
